# Supplementary material for: Temporal Alignment Networks for Long-term Video
Source: arXiv:2204.02968 source file (2022-04-06)
Supplement: Supplementary file 1 [file appendix.tex]

\appendix
\section{Appendix}
